# Supplementary material for: Backstepping Temporal Difference Learning
Source: arXiv:2302.09875 source file (2025-04-18)
Supplement: Supplementary file 1 [file dummy.tex]

\begin{table}[H]
\begin{tabular}{|l||*{5}{c|}}\hline
\backslashbox{Env}{$\eta$}
&\makebox[3em]{0.1}&\makebox[3em]{0.5}&\makebox[3em]{1}
&\makebox[3em]{4}&\makebox[3em]{8}\\\hline\hline
Boyan-BoyanRep &0.676 \pm 0.618 &0.86 \pm 0.526 &0.887 \pm 0.518 &0.91 \pm 0.511 &0.917 \pm 0.508\\\hline
RandomWalk-DependentRep &0.022 \pm 0.025 &0.024 \pm 0.027 &0.024 \pm 0.028 &0.024 \pm 0.029 &0.025 \pm 0.029\\\hline
RandomWalk-InvertedRep &0.063 \pm 0.054 &0.064 \pm 0.055 &0.065 \pm 0.056 &0.065 \pm 0.056 &0.066 \pm 0.055\\\hline
RandomWalk-TabularRep &0.039 \pm 0.035 &0.042 \pm 0.036 &0.043 \pm 0.037 &0.044 \pm 0.037 &0.045 \pm 0.037\\\hline
Baird-BairdRep & 9e+3 \pm 2e+5 &0.158 \pm 0.809 &0.093 \pm 0.655 &0.068 \pm 0.599 &8e+51 \pm 4e+53
 \\\hline
\end{tabular}
\hfill
\centering
\caption{TDRC, \(\beta=0.1\)}
\end{table}

\begin{table}[H]
\begin{tabular}{|l||*{5}{c|}}\hline
\backslashbox{Env}{$\eta$}
&\makebox[3em]{0.1}&\makebox[3em]{0.5}&\makebox[3em]{1}
&\makebox[3em]{4}&\makebox[3em]{8}\\\hline\hline
Boyan-BoyanRep &1.824 \pm 0.236 &1.364 \pm 0.353 &0.893 \pm 0.526 &1.357 \pm 0.493 &2.794 \pm 0.944\\\hline
\textbf{RandomWalk-DependentRep} &0.031 \pm 0.037 &0.026 \pm 0.031 &0.023 \pm 0.025 &0.039 \pm 0.024 &0.072 \pm 0.042\\\hline
\textbf{RandomWalk-InvertedRep} &0.144 \pm 0.04 &0.091 \pm 0.055 &0.059 \pm 0.055 &0.05 \pm 0.036 &0.083 \pm 0.041\\\hline
RandomWalk-TabularRep &0.068 \pm 0.046 &0.052 \pm 0.04 &0.047 \pm 0.035 &0.09 \pm 0.045 &0.166 \pm 0.081\\\hline
{\color{blue}Baird-BairdRep} &0.105 \pm 0.658 &0.108 \pm 0.665 &0.124 \pm 0.689 &0.298 \pm 1.067 &0.576 \pm 1.846\\\hline
\end{tabular}
\hfill
\centering
\caption{BackStepping TD, \(\beta=0.1\)}
\end{table}

\begin{table}[H]
\begin{tabular}{|l||*{5}{c|}}\hline
\backslashbox{Env}{$\eta$}
&\makebox[3em]{0.1}&\makebox[3em]{0.5}&\makebox[3em]{1}
&\makebox[3em]{4}&\makebox[3em]{8}\\\hline\hline
Boyan-BoyanRep & 1.208\pm 0.425 & 1.201 \pm 0.428 & 1.199 \pm 0.429 & 1.187 \pm 0.431& 1.167\pm 0.433\\\hline
RandomWalk-DependentRep &0.02 \pm 0.025& 0.02 \pm 0.025& 0.012 \pm 0.025 & 0.02 \pm 0.026 & 0.021 \pm 0.025 \\\hline
RandomWalk-InvertedRep &0.059\pm 0.055& 0.059\pm 0.056 & 0.060 \pm 0.056&  0.060 \pm 0.0552& 0.061\pm 0.055\\\hline
RandomWalk-TabularRep & 0.035 \pm 0.036 & 0.036 \pm 0.037 & 0.036 \pm 0.037 &  0.036 \pm 0.037 & 0.036 \pm 0.037 \\\hline
Baird-BairdRep & 9.360 \pm 7.651 & 0.126 \pm 0.734 & 0.010 \pm 0.652 & 0.087 \pm 0.622 & 0.090 \pm 0.632 \\\hline
\end{tabular}
\hfill
\centering
\caption{TDRC, \(\beta=1\)}
\end{table}

\begin{table}[H]
\begin{tabular}{|l||*{5}{c|}}\hline
\backslashbox{Env}{$\eta$}
&\makebox[3em]{0.1}&\makebox[3em]{0.5}&\makebox[3em]{1}
&\makebox[3em]{4}&\makebox[3em]{8}\\\hline\hline
\textbf{Boyan-BoyanRep} & 1.561\pm 0.537 & 1.011 \pm 0.647 & 1.198 \pm 0.437 & 2.550 \pm 0.912& 4.025 \pm 1.614\\\hline
RandomWalk-DependentRep & 0.050 \pm 0.043 &0.023 \pm 0.032 & 0.020 \pm 0.025& 0.029 \pm 0.018 & 0.045 \pm 0.023\\\hline
\textbf{RandomWalk-InvertedRep} & 0.177 \pm 0.030 & 0.096 \pm 0.055 & 0.059 \pm 0.553& 0.040 \pm 0.033 & 0.054 \pm 0.029\\\hline
RandomWalk-TabularRep & 0.099 \pm 0.050 & 0.047 \pm 0.045 & 0.037 \pm 0.036 & 0.058 \pm 0.030  & 0.098 \pm 0.047\\ \hline
{\color{blue}Baird-BaridRep} & 0.100 \pm 0.655 & 0.095\pm 0.653 & 0.104 \pm 0.660 & 0.199 \pm 0.875 & 0.661\pm  2.473 \\\hline
\end{tabular}
\hfill
\centering
\caption{BacksteppingTD, \(\beta=1\)}
\end{table}

\begin{table}[H]
\begin{tabular}{|l||*{5}{c|}}\hline
\backslashbox{Env}{$\eta$}
&\makebox[3em]{0.1}&\makebox[3em]{0.5}&\makebox[3em]{1}
&\makebox[3em]{4}&\makebox[3em]{8}\\\hline\hline
Boyan-BoyanRep &1.343 \pm 0.401 &  1.341 \pm 0.402 & 1.339 \pm 0.402 & 1.325 \pm 0.403 &1.299 \pm 0.405 \\\hline
RandomWalk-DependentRep & 0.019 \pm 0.025 & 0.019 \pm 0.025 & 0.019 \pm 0.025 & 0.02 \pm 0.025 & 0.021 \pm 0.025 \\\hline
RandomWalk-InvertedRep & 0.059 \pm 0.055 & 0.059 \pm 0.055 & 0.059 \pm 0.055&0.06 \pm 0.055 & 0.061 \pm 0.054\\\hline
RandomWalk-TabularRep & 0.035 \pm 0.036 &0.035 \pm 0.036 &0.035 \pm 0.036 &0.035 \pm 0.036 &0.036 \pm 0.036\\ \hline
Baird-BaridRep & 0.814 \pm 1.65 &0.131 \pm 0.738 &0.116 \pm 0.684 &0.113 \pm 0.664 &0.12 \pm 0.688
 \\\hline
\end{tabular}
\hfill
\centering
\caption{TDRC, \(\beta=2\)}
\end{table}

\begin{table}[H]
\begin{tabular}{|l||*{5}{c|}}\hline
\backslashbox{Env}{$\eta$}
&\makebox[3em]{0.1}&\makebox[3em]{0.5}&\makebox[3em]{1}
&\makebox[3em]{4}&\makebox[3em]{8}\\\hline\hline
\textbf{Boyan-BoyanRep} & 1.772\pm 0.508& 1.190 \pm 0.579& 1.340 \pm 0.407&  2.648 \pm 0.955 & 4.109 \pm  1.672\\\hline
RandomWalk-DependentRep & 0.057 \pm 0.044 & 0.023 \pm 0.032
 &0.019 \pm 0.025 & 0.028 \pm 0.018 & 0.041 \pm 0.022 \\\hline
\textbf{RandomWalk-InvertedRep} &0.18 \pm 0.029 &0.096 \pm 0.055 & 0.059 \pm 0.055& 0.04 \pm 0.034 & 0.051 \pm 0.029\\\hline
RandomWalk-TabularRep & 0.108 \pm 0.049 &0.046 \pm 0.046 &0.036 \pm 0.036 &0.052 \pm 0.028 &0.084 \pm 0.04\\ \hline
\textbf{Baird-BaridRep} & 0.115 \pm 0.68 &0.109 \pm 0.681 &0.122 \pm 0.689 &0.19 \pm 0.903 &2.118 \pm 12.756\\\hline
\end{tabular}
\hfill
\centering
\caption{BacksteppingTD, \(\beta=2\)}
\end{table}

\begin{table}[H]
\begin{tabular}{|l||*{5}{c|}}\hline
\backslashbox{Env}{$\eta$}
&\makebox[3em]{0.1}&\makebox[3em]{0.5}&\makebox[3em]{1}
&\makebox[3em]{4}&\makebox[3em]{8}\\\hline\hline
Boyan-BoyanRep &1.995 \pm 0.422 &1.297 \pm 0.543 &1.418 \pm 0.395 &2.698 \pm 0.976 &4.155 \pm 1.696\\\hline
RandomWalk-DependentRep &0.062 \pm 0.044 &0.023 \pm 0.032 &0.019 \pm 0.024 &0.027 \pm 0.018 &0.039 \pm 0.021\\\hline
RandomWalk-InvertedRep &0.182 \pm 0.028 &0.096 \pm 0.055 &0.059 \pm 0.055 &0.04 \pm 0.034 &0.05 \pm 0.029\\\hline
RandomWalk-TabularRep &0.114 \pm 0.049 &0.045 \pm 0.046 &0.035 \pm 0.036 &0.049 \pm 0.027 &0.074 \pm 0.035\\\hline
Baird-BairdRep &0.148 \pm 0.748 &0.154 \pm 0.764 &0.195 \pm 0.791 &0.414 \pm 1.559 &1e+16 \pm 3e+17\\\hline
\end{tabular}
\hfill
\centering
\caption{BacksteppingTD, \(\beta=4\)}
\end{table}

\begin{table}[H]
\begin{tabular}{c c c}\hline
\backslashbox{Env}{Algorithms}
&\makebox[3em]{TDRC}&\makebox[3em]{BTDRC}\\\hline
Boyan-BoyanRep & 0.336 \pm 0.024 & 0.548 \pm 0.02  \\\hline
RandomWalk-DependentRep & 0.01 \pm 0.005 & 0.008 \pm 0.004\\\hline
RandomWalk-InvertedRep & 0.014 \pm 0.004 & 0.015 \pm 0.005\\\hline
RandomWalk-TabularRep & 0.021 \pm 0.008 & 0.027 \pm 0.009\\\hline
Baird-BairdRep & 0.009 \pm 0.0 & 0.008 \pm 0.0\\\hline
\end{tabular}
\hfill
\centering
\caption{\(\beta=0.1\), last error, best case}
\end{table}

\begin{table}[H]
\begin{tabular}{c c c}\hline
\backslashbox{Env}{Algorithms}
&\makebox[3em]{TDRC}&\makebox[3em]{BTDRC}\\\hline
Boyan-BoyanRep & 1.312 \pm 0.054  & 0.659 \pm 0.023 \\\hline
RandomWalk-DependentRep & 0.011 \pm 0.005 & 0.009 \pm 0.003 \\\hline
\textbf{RandomWalk-InvertedRep} &0.014 \pm 0.005 &0.014 \pm 0.005\\\hline
RandomWalk-TabularRep & 0.02 \pm 0.008 &0.018 \pm 0.007 \\\hline
\textbf{Baird-BairdRep} & 0.019 \pm 0.003 &  0.0 \pm 0.0 \\\hline
\end{tabular}
\hfill
\centering
\caption{\(\beta=1\), last error, best case}
\end{table}

\begin{table}[H]
\begin{tabular}{c c c}\hline
\backslashbox{Env}{Algorithms}
&\makebox[3em]{TDRC}&\makebox[3em]{BTDRC}\\\hline
Boyan-BoyanRep & 1.52 \pm 0.059 & 0.957 \pm 0.028 \\\hline
RandomWalk-DependentRep & 0.011 \pm 0.005 & 0.009 \pm 0.004 \\\hline
RandomWalk-InvertedRep & 0.014 \pm 0.005 & 0.015 \pm 0.005\\\hline
RandomWalk-TabularRep & 0.02 \pm 0.008 & 0.017 \pm 0.006 \\\hline
Baird-BairdRep & 0.027 \pm 0.006 & 0.0 \pm 0.0\\\hline
\end{tabular}
\hfill
\centering
\caption{\(\beta=2\), last error, best case}
\end{table}

\begin{table}[H]
\begin{tabular}{c c c}\hline
\backslashbox{Env}{Algorithms}
&\makebox[3em]{TDRC}&\makebox[3em]{BTDRC}\\\hline
Boyan-BoyanRep & 1.619 \pm 0.062 & 1.133 \pm 0.03\\\hline
RandomWalk-DependentRep & 0.012 \pm 0.005 & 0.009 \pm 0.004\\\hline
RandomWalk-InvertedRep & 0.015 \pm 0.006 & 0.015 \pm 0.006 \\\hline
RandomWalk-TabularRep & 0.02 \pm 0.008 & 0.016 \pm 0.006\\\hline
Baird-BairdRep & 0.036 \pm 0.01 & 0.0 \pm 0.0 \\\hline
\end{tabular}
\hfill
\centering
\caption{\(\beta=4\), last error, best case}
\end{table}

\begin{table}[H]
\begin{tabular}{|l||*{5}{c|}}\hline
\backslashbox{Env}{$\eta$}
&\makebox[3em]{0.1}&\makebox[3em]{0.5}&\makebox[3em]{1}
&\makebox[3em]{4}&\makebox[3em]{8}\\\hline\hline
Boyan-BoyanRep &0.336 \pm 0.024 &0.535 \pm 0.02 &0.551 \pm 0.019 &0.569 \pm 0.018 &0.581 \pm 0.018\\\hline
RandomWalk-DependentRep &0.011 \pm 0.005 &0.011 \pm 0.005 &0.01 \pm 0.005 &0.01 \pm 0.005 &0.011 \pm 0.006\\\hline
RandomWalk-InvertedRep &0.016 \pm 0.005 &0.015 \pm 0.004 &0.014 \pm 0.004 &0.015 \pm 0.004 &0.016 \pm 0.004\\\hline
RandomWalk-TabularRep &0.021 \pm 0.008 &0.021 \pm 0.008 &0.022 \pm 0.008 &0.023 \pm 0.009 &0.023 \pm 0.01\\\hline
Baird-BairdRep &91662.59 \pm 110360.673 &0.009 \pm 0.0 &0.009 \pm 0.0 &0.009 \pm 0.001 &4e+53 \pm 3e+54\\\hline
\end{tabular}
\hfill
\centering
\caption{TDRC, \(\beta=0.1\) last error}
\end{table}

\begin{table}[H]
\begin{tabular}{|l||*{5}{c|}}\hline
\backslashbox{Env}{$\eta$}
&\makebox[3em]{0.1}&\makebox[3em]{0.5}&\makebox[3em]{1}
&\makebox[3em]{4}&\makebox[3em]{8}\\\hline\hline
Boyan-BoyanRep &1.374 \pm 0.053 &1.366 \pm 0.052 &1.362 \pm 0.052 &1.342 \pm 0.053 &1.312 \pm 0.054\\\hline
RandomWalk-DependentRep &0.011 \pm 0.005 &0.011 \pm 0.005 &0.011 \pm 0.005 &0.012 \pm 0.006 &0.013 \pm 0.006\\\hline
RandomWalk-InvertedRep &0.014 \pm 0.005 &0.014 \pm 0.005 &0.014 \pm 0.005 &0.015 \pm 0.005 &0.017 \pm 0.005\\\hline
RandomWalk-TabularRep &0.02 \pm 0.008 &0.02 \pm 0.008 &0.02 \pm 0.008 &0.02 \pm 0.009 &0.021 \pm 0.009\\\hline
Baird-BairdRep &12.428 \pm 13.254 &0.02 \pm 0.004 &0.019 \pm 0.003 &0.019 \pm 0.003 &0.021 \pm 0.007\\\hline
\end{tabular}
\hfill
\centering
\caption{TDRC, \(\beta=1\) last error}
\end{table}

\begin{table}[H]
\begin{tabular}{|l||*{5}{c|}}\hline
\backslashbox{Env}{$\eta$}
&\makebox[3em]{0.1}&\makebox[3em]{0.5}&\makebox[3em]{1}
&\makebox[3em]{4}&\makebox[3em]{8}\\\hline\hline
Boyan-BoyanRep &0.887 \pm 0.006 &0.659 \pm 0.023 &1.362 \pm 0.053 &4.056 \pm 0.218 &6.51 \pm 0.377\\\hline
RandomWalk-DependentRep &0.009 \pm 0.003 &0.009 \pm 0.004 &0.012 \pm 0.005 &0.026 \pm 0.013 &0.041 \pm 0.02\\\hline
RandomWalk-InvertedRep &0.134 \pm 0.002 &0.031 \pm 0.003 &0.014 \pm 0.005 &0.03 \pm 0.012 &0.047 \pm 0.02\\\hline
RandomWalk-TabularRep &0.045 \pm 0.002 &0.018 \pm 0.007 &0.022 \pm 0.01 &0.054 \pm 0.026 &0.093 \pm 0.042\\\hline
Baird-BairdRep &0.009 \pm 0.001 &0.015 \pm 0.002 &0.023 \pm 0.005 &0.012 \pm 0.007 &0.0 \pm 0.0\\\hline
\end{tabular}
\hfill
\centering
\caption{BacksteppingTD, \(\beta=1\) last error}
\end{table}

\begin{table}[H]
\begin{tabular}{|l||*{5}{c|}}\hline
\backslashbox{Env}{$\eta$}
&\makebox[3em]{0.1}&\makebox[3em]{0.5}&\makebox[3em]{1}
&\makebox[3em]{4}&\makebox[3em]{8}\\\hline\hline
Boyan-BoyanRep &1.59 \pm 0.059 &1.586 \pm 0.059 &1.583 \pm 0.059 &1.56 \pm 0.059 &1.52 \pm 0.059\\\hline
RandomWalk-DependentRep &0.012 \pm 0.005 &0.011 \pm 0.005 &0.011 \pm 0.005 &0.012 \pm 0.006 &0.013 \pm 0.006\\\hline
RandomWalk-InvertedRep &0.015 \pm 0.005 &0.014 \pm 0.005 &0.014 \pm 0.005 &0.015 \pm 0.005 &0.017 \pm 0.005\\\hline
RandomWalk-TabularRep &0.02 \pm 0.008 &0.02 \pm 0.008 &0.02 \pm 0.008 &0.02 \pm 0.008 &0.02 \pm 0.008\\\hline
Baird-BairdRep &0.038 \pm 0.018 &0.028 \pm 0.007 &0.027 \pm 0.006 &0.027 \pm 0.005 &0.03 \pm 0.011\\\hline
\end{tabular}
\hfill
\centering
\caption{TDRC, \(\beta=2\) last error}
\end{table}

\begin{table}[H]
\begin{tabular}{|l||*{5}{c|}}\hline
\backslashbox{Env}{$\eta$}
&\makebox[3em]{0.1}&\makebox[3em]{0.5}&\makebox[3em]{1}
&\makebox[3em]{4}&\makebox[3em]{8}\\\hline\hline
Boyan-BoyanRep &0.992 \pm 0.006 &0.957 \pm 0.028 &1.582 \pm 0.059 &4.215 \pm 0.226 &6.65 \pm 0.386\\\hline
RandomWalk-DependentRep &0.011 \pm 0.002 &0.009 \pm 0.004 &0.012 \pm 0.005 &0.025 \pm 0.012 &0.037 \pm 0.018\\\hline
RandomWalk-InvertedRep &0.138 \pm 0.001 &0.031 \pm 0.003 &0.015 \pm 0.005 &0.03 \pm 0.012 &0.044 \pm 0.019\\\hline
RandomWalk-TabularRep &0.05 \pm 0.002 &0.017 \pm 0.006 &0.021 \pm 0.009 &0.048 \pm 0.022 &0.079 \pm 0.034\\\hline
Baird-BairdRep &0.011 \pm 0.001 &0.021 \pm 0.002 &0.031 \pm 0.007 &0.0 \pm 0.0 &0.0 \pm 0.002\\\hline
\end{tabular}
\hfill
\centering
\caption{BacksteppingTD, \(\beta=2\) last error}
\end{table}

\begin{table}[H]
\begin{tabular}{|l||*{5}{c|}}\hline
\backslashbox{Env}{$\eta$}
&\makebox[3em]{0.1}&\makebox[3em]{0.5}&\makebox[3em]{1}
&\makebox[3em]{4}&\makebox[3em]{8}\\\hline\hline
Boyan-BoyanRep &1.711 \pm 0.062 &1.708 \pm 0.062 &1.704 \pm 0.062 &1.676 \pm 0.063 &1.619 \pm 0.062\\\hline
RandomWalk-DependentRep &0.012 \pm 0.005 &0.012 \pm 0.005 &0.012 \pm 0.005 &0.012 \pm 0.006 &0.013 \pm 0.006\\\hline
RandomWalk-InvertedRep &0.015 \pm 0.006 &0.015 \pm 0.006 &0.015 \pm 0.006 &0.016 \pm 0.006 &0.017 \pm 0.006\\\hline
RandomWalk-TabularRep &0.02 \pm 0.008 &0.02 \pm 0.008 &0.02 \pm 0.008 &0.02 \pm 0.008 &0.02 \pm 0.008\\\hline
Baird-BairdRep &0.039 \pm 0.017 &0.036 \pm 0.011 &0.036 \pm 0.01 &0.038 \pm 0.01 &0.042 \pm 0.021\\\hline
\end{tabular}
\hfill
\centering
\caption{TDRC, \(\beta=4\) last error}
\end{table}

\begin{table}[H]
\begin{tabular}{|l||*{5}{c|}}\hline
\backslashbox{Env}{$\eta$}
&\makebox[3em]{0.1}&\makebox[3em]{0.5}&\makebox[3em]{1}
&\makebox[3em]{4}&\makebox[3em]{8}\\\hline\hline
Boyan-BoyanRep &1.294 \pm 0.006 &1.133 \pm 0.03 &1.704 \pm 0.062 &4.296 \pm 0.231 &6.719 \pm 0.39\\\hline
RandomWalk-DependentRep &0.013 \pm 0.002 &0.009 \pm 0.004 &0.012 \pm 0.005 &0.024 \pm 0.012 &0.035 \pm 0.017\\\hline
RandomWalk-InvertedRep &0.14 \pm 0.001 &0.031 \pm 0.003 &0.015 \pm 0.006 &0.03 \pm 0.012 &0.042 \pm 0.018\\\hline
RandomWalk-TabularRep &0.054 \pm 0.002 &0.016 \pm 0.006 &0.021 \pm 0.009 &0.043 \pm 0.019 &0.069 \pm 0.028\\\hline
Baird-BairdRep &0.014 \pm 0.001 &0.034 \pm 0.005 &0.04 \pm 0.011 &0.0 \pm 0.0 &2e+17 \pm 1e+18\\\hline
\end{tabular}
\hfill
\centering
\caption{BacksteppingTD, \(\beta=4\) last error}
\end{table}
